# Supplementary material for: PI-HMR: Towards Robust In-bed Temporal Human Shape Reconstruction with Contact Pressure Sensing
Source: arXiv:2503.00068 source file (2025-03-22)
Supplement: Supplementary file 1 [file X_suppl.tex]

\clearpage
\setcounter{page}{1}
\maketitlesupplementary

% 使用TIP的原因
% 不使用仿真数据的原因

\section{More experiments}

\subsection{Comparison with other modalities}
hello

\setlength{\aboverulesep}{0pt}
\setlength{\belowrulesep}{0pt}
\begin{table*}[ht]
\centering
\begin{tabular}{l|c|c|cccc|cc}
\toprule[2pt]
Method       & Input             & Modalities                & MPJPE & MPJPE-P & PA-MPJPE & MPVE & Accel & Acc-Error \\
\hline
CLIFF        &  image                     & \multirow{3}{*}{RGB} &       &         &          &      &       &           \\ \cline{1-2} \cline{4-9}
TCMR         & \multirow{2}{*}{sequence}     &                    &       &         &          &      &       &           \\
MPS-NET      &                        &                    &       &         &          &      &       &           \\
\hline
BodyMAP      & \multirow{2}{*}{image} & \multirow{2}{*}{D + P} &       &         &          &      &       &           \\
BodyMAP-WS   &                        &                    &       &         &          &      &       &           \\
\hline
PI-HMR-Basic (ours)       &                        &                    &       &         &          &      &       &           \\
PI-HMR (ours)       &                        &                    &       &         &          &      &       &           \\
PI-HMR + TTO (ours) &                        &                    &       &         &          &      &       &           \\
\bottomrule[2pt]
\end{tabular}
\end{table*}
